# Supplementary material for: Open-World Stereo Video Matching with Deep RNN
Source: arXiv:1808.03959 source file (2018-08-12)
Supplement: Supplementary file 1 [file 1546_supp.pdf]

# Open-World Stereo Video Matching with Deep RNN

Yiran Zhong[1,3,4], Hongdong Li[1,3], Yuchao Dai[2]

[1] Australian National University, Australia
[2] Northwestern Polytechnical University, China
[3] Australian Centre for Robotic Vision, Australia
[4] Data61 CSIRO, Australia
{yiran.zhong,hongdong.li}@anu.edu.au daiyuchao@nwpu.edu.cn

**Abstract.** In this supplementary material, we provide detailed network design of our OpenStereoNet, including network structure, layer size and key parameters. We also provide more experimental results, explaining the effect of the network "prime" process. We perform additional experiments on our Convolutional-LSTM modules, specifically to demonstrate its ability in capturing and exploiting temporal smoothness property of a continuous video. We will make our code publicly available.

## 1 Network Design Details

Our network architecture consists of 4 blocks: (1) Feature-Net, (2) Feature-Volume construction, (3) Match-Net and (4) Projection layer. Detailed structure of our network is given in Table 1.

## 2 The Effect of Network *Prime* Process

The purpose of network prime is to expose our network to a number of typical natural images in order to train the Feature-Net to produce reasonable feature maps. This process is performed only once. To analyze the effect of our network *prime* process, we visualize the first three layers of the obtained feature maps before, and after the prime process, as shown in Fig. 1.

## 3 Experimental results on the KITTI stereo dataset

We have conducted additional experiments on the KITTI 2015 stereo dataset and the results are reported in Table 1. To handle the static and noncontinuous stereo frames, we augmented each stereo pair to a stereo video sequence. By comparing with supervised method [4] (using a model that was trained on SceneFlow dataset for a fair comparison), our method again achieves the best performance.

| layer | k | s | chns | in | out | input |
|---|---|---|---|---|---|---|
| **Feature-Net** | | | | | | |
| conv1 | 5 | 2 | 3/32 | 1 | 2 | image |
| conv2 | 3 | 1 | 32/32 | 2 | 2 | conv1 |
| conv3 | 3 | 1 | 32/32 | 2 | 2 | conv2 |
| add1 | 1 | 1 | 64/32 | 2 | 2 | conv1+conv3 |
| conv4 | 3 | 1 | 32/32 | 2 | 2 | add1 |
| conv5 | 3 | 1 | 32/32 | 2 | 2 | conv4 |
| add2 | 1 | 1 | 64/32 | 2 | 2 | conv3+conv5 |
| conv6 | 3 | 1 | 32/32 | 2 | 2 | add2 |
| conv7 | 3 | 1 | 32/32 | 2 | 2 | conv6 |
| add3 | 1 | 1 | 64/32 | 2 | 2 | conv5+conv7 |
| conv8 | 3 | 1 | 32/32 | 2 | 2 | add3 |
| conv9 | 3 | 1 | 32/32 | 2 | 2 | conv8 |
| add4 | 1 | 1 | 64/32 | 2 | 2 | conv7+conv9 |
| conv10 | 3 | 1 | 32/32 | 2 | 2 | add4 |
| conv11 | 3 | 1 | 32/32 | 2 | 2 | conv10 |
| add5 | 1 | 1 | 64/32 | 2 | 2 | conv9+conv11 |
| conv12 | 3 | 1 | 32/32 | 2 | 2 | add5 |
| conv13 | 3 | 1 | 32/32 | 2 | 2 | conv12 |
| add6 | 1 | 1 | 64/32 | 2 | 2 | conv11+conv13 |
| conv14 | 3 | 1 | 32/32 | 2 | 2 | add6 |
| conv15 | 3 | 1 | 32/32 | 2 | 2 | conv14 |
| add7 | 1 | 1 | 64/32 | 2 | 2 | conv13+conv15 |
| conv16 | 3 | 1 | 32/32 | 2 | 2 | add7 |
| conv17 | 3 | 1 | 32/32 | 2 | 2 | conv16 |
| convlstm | 3 | 1 | 32/32 | 2 | 2 | conv17,hidden |
| conv18* | 3 | 1 | 32/32 | 2 | 2 | convlstm+conv17 |
| **Match-Net** | | | | | | |
| conv_1_1 | 3 | 1 | 64/32 | 2 | 2 | feature volume |
| conv_1_2 | 3 | 1 | 32/32 | 2 | 2 | conv_1_1 |
| conv_2_1 | 3 | 2 | 64/64 | 2 | 4 | feature volume |
| conv_2_2 | 3 | 1 | 64/64 | 4 | 4 | conv_2_1 |
| conv_2_3 | 3 | 1 | 64/64 | 4 | 4 | conv_2_2 |
| conv_3_1 | 3 | 2 | 64/64 | 4 | 8 | conv_2_1 |
| conv_3_2 | 3 | 1 | 64/64 | 8 | 8 | conv_3_1 |
| conv_3_3 | 3 | 1 | 64/64 | 8 | 8 | conv_3_2 |
| conv_4_1 | 3 | 2 | 64/64 | 8 | 16 | conv_3_1 |
| conv_4_2 | 3 | 1 | 64/64 | 16 | 16 | conv_4_1 |
| conv_4_3 | 3 | 1 | 64/64 | 16 | 16 | conv_4_2 |
| conv_5_1 | 3 | 2 | 64/128 | 16 | 32 | conv_4_1 |
| conv_5_2 | 3 | 1 | 128/128 | 32 | 32 | conv_5_1 |
| conv_5_3 | 3 | 1 | 128/128 | 32 | 32 | conv_5_2 |
| conv_lstm | 3 | 1 | 128/128 | 32 | 32 | conv_5_3 |
| deconv_5_1 | 3 | 2 | 128/64 | 16 | 16 | conv_lstm,hidden |
| deconv_4_1 | 3 | 2 | 64/64 | 8 | 8 | conv_4_3 + deconv_5_1 |
| deconv_3_1 | 3 | 2 | 64/64 | 4 | 4 | conv_3_3 + deconv_4_1 |
| deconv_2_1 | 3 | 2 | 64/32 | 2 | 2 | conv_2_3 + deconv_3_1 |
| **Projection layer** | | | | | | |
| proj* | 3 | 2 | 32/1 | 1 | 1 | conv_1_2 + deconv_2_1 |

**Table 1. Our network structure. k**, **s**, **chns** represent the kernel size, stride and the number of the input and the output channels. **in**, **out** are the downscaling factor of each layer relative to the input. "+" represents element-wise sum. All the convolution layers are followed by a batch normalization and a relu activation except the layer marked with *. "hidden" means the hidden layer of a cLSTM layer.

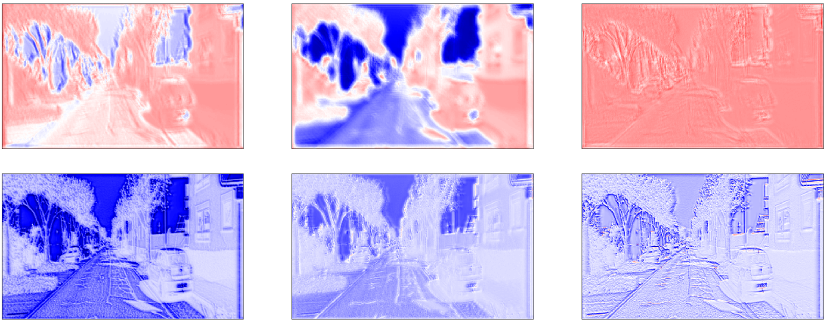

**Fig. 1. Feature visualization.** Each row shows the first 3 output feature maps (color coded) from our Feature-Net. The top row shows the features without network prime process while the bottom row shows the one after applying the network prime process. We can observe that the network prime process allows the network to capture more local details such as edges and corners while the original one is more blurry and smooth.

| Methods | Abs Rel | Sq Rel | RMSE | RMSE log | D1_all | $\delta < 1.25$ |
|---|---|---|---|---|---|---|
| SPS-st (ECCV 2014) | 0.078 | 1.556 | 5.209 | 0.149 | 5.280 | 0.954 |
| GC-Net (ICCV 2017) | 0.099 | 0.987 | 4.475 | 0.157 | 18.674 | 0.929 |
| LRC Stereo (CVPR 2017) | 0.068 | 0.835 | 4.392 | 0.146 | 9.194 | 0.942 |
| Unstereo (ICCV 2017) | - | - | - | - | 9.510 | - |
| Ours | **0.056** | **0.692** | **3.176** | **0.125** | **5.140** | **0.967** |

**Table 2.** Performance comparison between our method and state-of-the-art methods on KITTI 2015.

## 4 Reshuffled VS Original Stereo Video Matching

Our cLSTM units are intended to memorize and to exploit temporal dynamics contained in a continuous stereo video sequence. In this section, we conduct experiments to analyze what if the input video is reshuffled in a temporally random order such that its temporal smoothness is totally destroyed.

Specifically, we feed the network with a randomly reshuffled video sequence. In this case, the temporal consistency assumption is violated and the learned temporal transition from previous frames will provide little help for the current input frame. In other words, the LSTM module will become less useful in this scenario. In Fig. 2, we compare our network's performance on the original video sequence and the reshuffled one, from which we can observe that: in terms of disparity MAE, our method achieves an error rate of 0.8819 pixels for the original sequential video and 1.1767 pixels for the randomly reshuffled video. The performance has dropped 33.43%, which demonstrates that our cLSTM units do memorize and exploit the temporal dynamics in continuous stereo video sequences.

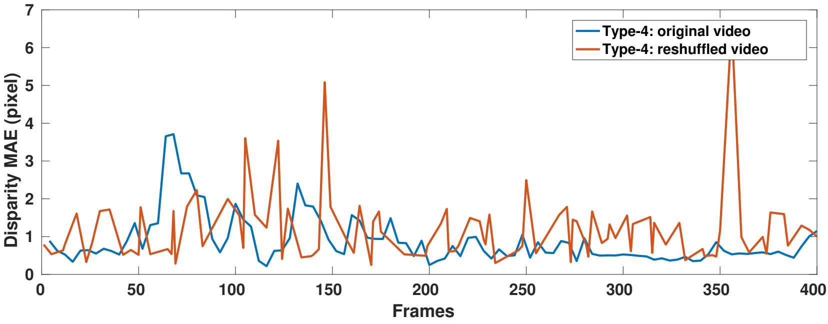


**Fig. 2. Comparing cLSTM for the reshuffled and the original video.** Our method achieves a disparity MAE of 1.1767 pixels for the randomly reshuffled stereo video sequence and 0.8819 pixels for the original continuous stereo video sequence.

## 5 Other Open-world Stereo Video Matching Results

We have also tested our OpenStereoNet on different open-world stereo matching tasks. In Fig. 3, we show the result from a simple stereo video captured by a Microsoft Surface Pro 10. In Fig-4, we show the results on a stereo video captured by a ZED stereo camera.

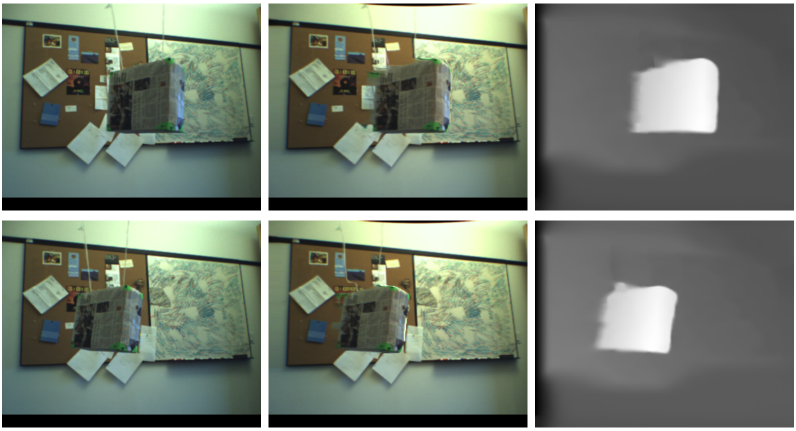

**Fig. 3. Our stereo matching results on a Microsoft surface stereo test video.** From left to right: input left image, our recovered left image and our estimated disparity map.

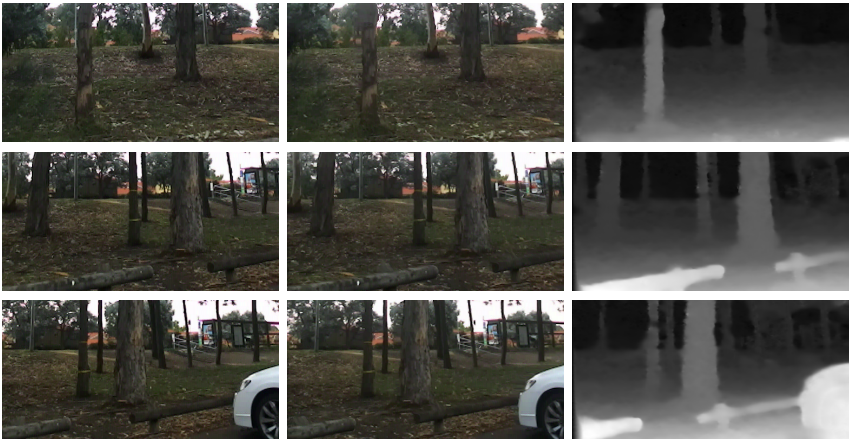

**Fig. 4. Our stereo matching results on a casual stereo video sequence captured by a Zed stereo camera.** From left to right: input left image, our recovered left image and our estimated disparity map.
